# Supplementary material for: Biorthogonal projected energies of a Gutzwiller similarity transformed Hamiltonian
Source: arXiv:1610.02053 ancillary file (2016-10-06)
Supplement: Supplementary file 1 [file Supplemental_Material.pdf]

# Supplemental information for "Biorthogonal projected energies of a Gutzwiller similarity transformed Hamiltonian"


**J M Wahlen-Strothman[1], G E Scuseria[1,2,3]**

[1]Department of Physics and Astronomy, Rice University, Houston, USA 77005
[2]Department of Chemistry, Rice University, Houston, USA 77005
[3]Department of Materials Science and NanoEngineering, Rice University, Houston, USA 77005


## Gutzwiller Hausdorff Series Resummation

We wish to show that

$$\begin{aligned} e^{-J}c^{\dagger}_{k\uparrow}e^{J} &= e^{-\alpha_k n_{k\downarrow}}c^{\dagger}_{k\uparrow}, \\ e^{-J}c^{\dagger}_{k\uparrow}e^{J} &= (1+(e^{-\alpha_k}-1)n_{k\downarrow})c^{\dagger}_{k\uparrow}. \end{aligned} \tag{1}$$

Expand in the commutator series

$$e^{-J}c^{\dagger}_{k\uparrow}e^{J} = c^{\dagger}_{p\uparrow} + \left[c^{\dagger}_{k\uparrow}, J\right] + \frac{1}{2}\left[\left[c^{\dagger}_{k\uparrow}, J\right], J\right] + ... \tag{2}$$

The first commutator is

$$\begin{aligned} \left[c^{\dagger}_{k\uparrow}, J\right] &= \sum_i \alpha_i \left[c^{\dagger}_{k\uparrow}, n_{i\uparrow}n_{\downarrow}\right] \\ &= -\alpha_k n_{k\downarrow}c^{\dagger}_{k\sigma}. \end{aligned} \tag{3}$$

The second commutator is

$$\begin{aligned} \left[\left[c^{\dagger}_{k\uparrow}, J\right], J\right] &= -\alpha_k n_{k\downarrow}\left[c^{\dagger}_{k\uparrow}, J\right] \\ &= (\alpha_k n_{k\downarrow})^2 c^{\dagger}_{k\uparrow} \\ &= \alpha_k^2 n_{k\downarrow}c^{\dagger}_{k\uparrow} \end{aligned} \tag{4}$$

From this, Eq. 2 is clearly resummable in two ways leading to the main results.

**UGST Energy, Amplitude, and Double-Occupancy Equations**

Here we use the notation,

$$\rho^{\alpha}_{ij} = \rho_{i\uparrow,j\uparrow}, \quad \rho^{\beta}_{ij} = \rho_{i\downarrow,j\downarrow}, \tag{5}$$

to represent the up and down one-particle transition spin densities of the UHF wavefunctions in the lattice basis. The Wick expansion holds for overlaps of determinants with different single particle bases as long as the proper transition density is used. ‡

$$E = -t\sum_{\langle ij\rangle}\Bigg(\Big(1+\xi^-_i\rho^{\beta}_{ii}+\xi^+_j\rho^{\beta}_{jj}+\xi^-_i\xi^+_j(\rho^{\beta}_{ii}\rho^{\beta}_{jj}-\rho^{\beta}_{ji}\rho^{\beta}_{ij})\Big)\rho^{\alpha}_{ji} + (\alpha \leftrightarrow \beta)\Bigg) + U\sum_i \rho^{\alpha}_{ii}\rho^{\beta}_{ii} \tag{6}$$

$$\begin{aligned} R_k = -t\sum_{\langle ij\rangle}\Bigg(\Big(&\rho^{\beta}_{kk}+\xi^-_i\langle\Phi'|n_{k\downarrow}n_{i\downarrow}|\Phi\rangle+\xi^+_j\langle\Phi'|n_{k\downarrow}n_{j\downarrow}|\Phi\rangle \\ &+\xi^-_i\xi^+_j\langle\Phi'|n_{k\downarrow}n_{i\downarrow}n_{j\downarrow}|\Phi\rangle\Big)(\delta_{ik}\rho^{\alpha}_{ki}+\rho^{\alpha}_{kk}\rho^{\alpha}_{ji}-\rho^{\alpha}_{jk}\rho^{\alpha}_{ki}) \\ &+(\alpha \leftrightarrow \beta)\Bigg) + U\sum_i\langle\Phi'|n_{k\uparrow}n_{i\uparrow}|\Phi\rangle\langle\Phi'|n_{k\downarrow}n_{i\downarrow}|\Phi\rangle \\ &-\rho^{\alpha}_{kk}\rho^{\beta}_{kk}E \end{aligned} \tag{7}$$

$$D = \Big(1-\sum_i z_i\rho^{\alpha}_{ii}\rho^{\beta}_{ii}\Big)\sum_j\rho^{\alpha}_{jj}\rho^{\beta}_{jj}+\sum_{ij}z_i\langle\Phi'|n_{i\uparrow}n_{j\uparrow}|\Phi\rangle\langle\Phi'|n_{i\downarrow}n_{j\downarrow}|\Phi\rangle \tag{8}$$

$$\langle\Phi'|n_{i\downarrow}n_{j\downarrow}|\Phi\rangle = \delta_{ij}\rho^{\beta}_{ji}+\rho^{\beta}_{ii}\rho^{\beta}_{jj}-\rho^{\beta}_{ji}\rho^{\beta}_{ij} \tag{9}$$

$$\begin{aligned} \langle\Phi'|n_{k\downarrow}n_{i\downarrow}n_{j\downarrow}|\Phi\rangle = \quad &\rho^{\beta}_{kk}(\delta_{ij}\rho^{\beta}_{ji}+\rho^{\beta}_{ii}\rho^{\beta}_{jj}-\rho^{\beta}_{ji}\rho^{\beta}_{ij}) \\ &+\rho^{\beta}_{ik}(\delta_{ik}\rho^{\beta}_{jj}-\delta_{jk}\rho^{\beta}_{ji}-\rho^{\beta}_{jj}\rho^{\beta}_{ki}+\rho^{\beta}_{ji}\rho^{\beta}_{kj}) \\ &+\rho^{\beta}_{jk}(\delta_{ij}\delta_{ik}-\delta_{ij}\rho^{\beta}_{ki}-\delta_{ik}\rho^{\beta}_{ij}+\delta_{jk}\rho^{\beta}_{ii}+\rho^{\beta}_{ij}\rho^{\beta}_{ki}-\rho^{\beta}_{ii}\rho^{\beta}_{kj}) \end{aligned} \tag{10}$$

‡ For details on matrix elements between non-orthogonal Slater determinants see: J.-P. Blaizot and G. Ripka, Quantum Theory of Finite Systems (MIT, Cambridge, MA, 1986). 93-97.

**Projection**

Expectation values taken with the projected wavefunctions are evaluated by numerically integrating over rotated states. The values for each point in the quadrature are calculated with transition densities constructed from a new set of coefficients based on the spin rotation. For example the energy,

$$E^s = \frac{\langle\Phi_L|\overline{H}P^s_{mm}|\Phi_R\rangle}{\langle\Phi_L|P^s_{mm}|\Phi_R\rangle}, \tag{11}$$

$$P^s_{mm} = \frac{2s+1}{2}\int_0^\pi \mathrm{d}\beta \sin\beta d^s_{mm}(\beta)e^{\mathrm{i}\beta S_y}, \tag{12}$$

can be evaluated at each integration point by rotating the right state with angle $\beta$,

$$|\Phi_R(\beta)\rangle = e^{i\beta S_y}|\Phi_R\rangle, \quad \Rightarrow \quad C^o_R(\beta) = e^{i\beta\frac{\sigma_y}{2}}C^o_R. \tag{13}$$

This is used to construct a new transition density and evaluate the expectation value for angle $\beta$,

$$S(\beta) = C^{o\dagger}_L C^o_R(\beta), \tag{14}$$

$$\rho(\beta) = C^o_R(\beta)S^{-1}(\beta)C^{o\dagger}_L, \tag{15}$$

$$\langle\Phi_L|\overline{H}P^s_{mm}|\Phi_R\rangle = \frac{2s+1}{2}\int_0^\pi \mathrm{d}\beta \sin\beta d^s_{mm}(\beta)\det(S(\beta))E[\rho(\beta)], \tag{16}$$

$$\langle\Phi_L|P^s_{mm}|\Phi_R\rangle = \frac{2s+1}{2}\int_0^\pi \mathrm{d}\beta \sin\beta d^s_{mm}(\beta)\det(S(\beta)), \tag{17}$$

where $E[\rho]$ is the energy functional (6).

**Data Tables**

The following tables contain calculated correlation energies, double occupancies, and reference data with coupled-cluster singles and doubles (CCSD), exact diagonalization (ED), auxiliary-field quantum Monte Carlo (AFQMC), density matrix embedding theory (DMET), density matrix renormalization group theory (DMRG), and diffusion Monte Carlo based on a fixed-node approximation (FN). Uncertainties for the last digit from the methods or thermodynamic limit extrapolations are given in parentheses.

**Table 1.** Correlation energies per site with respect to UHF for $4 \times 4$ Hubbard lattices with spin quantum numbers $s = m = 0$ and $N_o$ electrons.

| $N_o$ | $U$ | $E_{UHF}$ | $\Delta_{SUHF}$ | $\Delta_{UGST}$ | $\Delta_{SUGST}$ | $\Delta_{UCCSD}$ | $\Delta_{ED}$ [a] |
|---|---|---|---|---|---|---|---|
| 14 | 1 | -1.3277 | -0.0015 | -0.0074 | -0.0084 | -0.0085 | -0.0093 |
| 14 | 2 | -1.1644 | -0.0069 | -0.0271 | -0.0309 | -0.0309 | -0.0338 |
| 14 | 3 | -1.0138 | -0.0168 | -0.0540 | -0.0615 | -0.0606 | -0.0674 |
| 14 | 4 | -0.8808 | -0.0175 | -0.0813 | -0.0930 | -0.0907 | -0.1032 |
| 14 | 6 | -0.6988 | -0.0382 | -0.0979 | -0.1173 | -0.1083 | -0.1400 |
| 14 | 8 | -0.5921 | -0.0352 | -0.0877 | -0.1121 | -0.1056 | -0.1497 |
| 14 | 10 | -0.5227 | -0.0315 | -0.0799 | -0.1019 | -0.1022 | -0.1527 |
| 14 | 12 | -0.4819 | -0.0256 | -0.0689 | -0.0880 | -0.0869 | -0.1463 |
| 16 | 1 | -1.2909 | -0.0022 | -0.0066 | -0.0082 | -0.0077 | -0.0087 |
| 16 | 2 | -1.0973 | -0.0098 | -0.0224 | -0.0281 | -0.0252 | -0.0288 |
| 16 | 3 | -0.9267 | -0.0220 | -0.0393 | -0.0505 | -0.0435 | -0.0506 |
| 16 | 4 | -0.7854 | -0.0338 | -0.0494 | -0.0667 | -0.0552 | -0.0660 |
| 16 | 6 | -0.5862 | -0.0426 | -0.0475 | -0.0736 | -0.0590 | -0.0733 |
| 16 | 8 | -0.4619 | -0.0410 | -0.0354 | -0.0645 | -0.0536 | -0.0674 |
| 16 | 10 | -0.3792 | -0.0373 | -0.0250 | -0.0536 | -0.0477 | -0.0601 |
| 16 | 12 | -0.3208 | -0.0336 | -0.0178 | -0.0449 | -0.0426 | -0.0537 |

[a] Results taken from G. Fano, F. Ortolani, and A. Parola, Phys. Rev. B **42**, 6877 (1990)

**Table 2.** Correlation energies per site with respect to UHF for $10 \times 10$ lattices with average occupancy $n$.

| $n$ | $U$ | $E_{UHF}$ | $\Delta_{UGST}$ | $\Delta_{SUGST}$ | $\Delta_{UCCSD}$[a,b] | $\Delta_{TDL}$[a] | |
|---|---|---|---|---|---|---|---|
| 0.8 | 2 | -1.2678 | -0.0358 | -0.0361 | -0.0416 | AFQMC | -0.038(2) |
| | | | | | | DMET | -0.0384(4) |
| | | | | | | FN | -0.0366(7) |
| 0.8 | 4 | -0.9774 | -0.1061 | -0.1087 | -0.1151 | AFQMC | -0.133(3) |
| | | | | | | DMET | -0.131(2) |
| | | | | | | DMRG | -0.127(1) |
| | | | | | | FN | -0.1258(7) |
| 0.8 | 6 | -0.7933 | -0.1335 | -0.1373 | -0.1275 | DMET | -0.184(4) |
| | | | | | | FN | -0.174(1) |
| 0.8 | 8 | -0.6815 | -0.1386 | -0.1424 | -0.1431 | DMET | -0.20(3) |
| | | | | | | FN | -0.196(1) |
| 1.0 | 2 | -1.1354 | -0.0286 | -0.0302 | -0.0318 | AFQMC | -0.0409(2) |
| | | | | | | DMET | -0.0410(3) |
| | | | | | | DMRG | -0.041(1) |
| | | | | | | FN | -0.040(1) |
| 1.0 | 4 | -0.7970 | -0.0532 | -0.0572 | -0.0582 | AFQMC | -0.0633(2) |
| | | | | | | DMET | -0.0634(3) |
| | | | | | | DMRG | -0.0635(5) |
| | | | | | | FN | -0.0605(3) |
| 1.0 | 6 | -0.5927 | -0.0487 | -0.0537 | -0.0583 | AFQMC | -0.0641(3) |
| | | | | | | DMET | -0.0635(5) |
| | | | | | | DMRG | -0.0638(1) |
| | | | | | | FN | -0.0624(1) |
| 1.0 | 8 | -0.4659 | -0.0366 | -0.0417 | -0.0532 | AFQMC | -0.0588(2) |
| | | | | | | DMET | -0.058(1) |
| | | | | | | DMRG | -0.0582(1) |
| | | | | | | FN | -0.0573 |
| 1.0 | 12 | -0.3225 | -0.0181 | -0.0229 | -0.0422 | AFQMC | -0.0468(2) |
| | | | | | | DMET | -0.046(1) |
| | | | | | | DMRG | -0.0464(1) |
| | | | | | | FN | -0.0459 |

[a] Results taken from J. P. F. LeBlanc *et al.*, Phys. Rev. X **5**, 041041 (2015).
[b] Results taken from C. A. Jiménez-Hoyos and G. E. Scuseria, Phys. Rev. B **92**, 085101 (2015).

**Table 3.** SUGST correlation energies per site for $30 \times 30$ square lattices with average occupancy $n$.

| $n$ | $U$ | $E_{UHF}$ | $\Delta_{SUGST}$ | $\Delta_{UCCSD}$[a] | $\Delta_{TDL}$[a] | |
|---|---|---|---|---|---|---|
| 0.8 | 2 | -1.2602 | -0.0376 | -0.0463[b] | AFQMC | -0.046(2) |
| | | | | | DMET | -0.0460(4) |
| | | | | | FN | -0.0442(7) |
| 0.8 | 4 | -0.9762 | -0.1026 | -0.1106[b] | AFQMC | -0.134(3) |
| | | | | | DMET | -0.132(2) |
| | | | | | DMRG | -0.128(1) |
| | | | | | FN | -0.1270(7) |
| 0.8 | 6 | -0.7843 | -0.1416 | -0.1457[b] | DMET | -0.193(4) |
| | | | | | FN | -0.183(1) |
| 0.8 | 8 | -0.6772 | -0.1432 | -0.1461[b] | DMET | -0.20(3) |
| | | | | | FN | -0.200(1) |
| 1.0 | 2 | -1.1389 | -0.0310 | -0.0364(4) | AFQMC | -0.0374(2) |
| | | | | | DMET | -0.0375(3) |
| | | | | | DMRG | -0.037(1) |
| | | | | | FN | -0.036(1) |
| 1.0 | 4 | -0.7978 | -0.0530 | -0.0568[c] | AFQMC | -0.0625(2) |
| | | | | | DMET | -0.0626(3) |
| | | | | | DMRG | -0.0627(5) |
| | | | | | FN | -0.0597(3) |
| 1.0 | 6 | -0.5927 | -0.0492 | -0.0585[d] | AFQMC | -0.0641(3) |
| | | | | | DMET | -0.0635(5) |
| | | | | | DMRG | -0.0638(1) |
| | | | | | FN | -0.0624(1) |
| 1.0 | 8 | -0.4659 | -0.0371 | -0.0532[d] | AFQMC | -0.0588(2) |
| | | | | | DMET | -0.058(1) |
| | | | | | DMRG | -0.0582(1) |
| | | | | | FN | -0.0573 |
| 1.0 | 12 | -0.3225 | -0.0187 | -0.0422[d] | AFQMC | -0.0468(2) |
| | | | | | DMET | -0.046(1) |
| | | | | | DMRG | -0.0464(1) |
| | | | | | FN | -0.0459 |

[a] Results taken from J. P. F. LeBlanc *et al.*, Phys. Rev. X **5**, 041041 (2015).
[b]$10 \times 16$ lattice, [c]$14 \times 14$ lattice, [d]$10 \times 10$ lattice

**Table 4.** Average SUGST double occupancies per site for 30 × 30 square lattices at half-filling.

| $U$ | UHF | SUGST | UCCSD[a] | TDL[a] | |
|---|---|---|---|---|---|
| 2 | 0.2146 | 0.1943 | 0.194(2) | AFQMC | 0.1923(3) |
| | | | | DMET | 0.1913(4) |
| | | | | DMRG | 0.188(1) |
| | | | | FN | 0.198(1) |
| 4 | 0.1307 | 0.1282 | 0.1268[b] | AFQMC | 0.1261(2) |
| | | | | DMET | 0.1261(1) |
| | | | | DMRG | 0.126(1) |
| | | | | FN | 0.125(1) |
| 6 | 0.0789 | 0.0843 | 0.0807[c] | AFQMC | 0.0810(1) |
| | | | | DMET | 0.0810 |
| | | | | DMRG | 0.0809(3) |
| | | | | FN | 0.0803(2) |
| 8 | 0.0507 | 0.0568 | 0.0537[c] | AFQMC | 0.0540(1) |
| | | | | DMET | 0.0540 |
| | | | | DMRG | 0.0539(1) |
| | | | | FN | 0.0535(1) |
| 12 | 0.0252 | 0.0283 | 0.0267[c] | AFQMC | 0.0278(1) |
| | | | | DMET | 0.0278 |
| | | | | DMRG | 0.0278(1) |
| | | | | FN | 0.0278(2) |

[a] Results taken from J. P. F. LeBlanc *et al.*, Phys. Rev. X **5**, 041041 (2015).
[b]12 × 12 lattice, [c]10 × 10 lattice
